# Supplementary material for: Exploring the Efficiency of Renewable Energy-based Modular Data Centers at Scale
Source: arXiv:2406.02252 source file (2024-06-04)
Supplement: Supplementary file 1 [file appendix.tex]

\section{Appendix}
\label{sec:appendix}
% \jinghan{explain more information on why MIP is a good fit; explain more clearly about the MIP inputs}
Once we colocate all the \siteName{s} with renewable energy farms and group them into subgraphs, we now place VMs across these \siteName{s}. A straightforward approach to this could be heuristic-based, such as greedily placing VMs onto the \siteName{s} in the order of their resource availability. 
However, heuristic-based approaches could be suboptimal, especially when the power supply changes over time and different VMs also have different priorities and demands on the computing resources, as it is difficult for heuristic-based approaches to identify the best-matching \siteName{s} for each VM workload.

In \name{}, we formalize the VM placement and migration problem into an optimization problem using the Mixed-Integer Program (MIP) model~\cite{mip}, in addition to the heuristic-based approach. \name{} employs the MIP model because it can handle a large set of decision variables under different constraints, and explore the optimized choices by taking the dynamic patterns of variables into the consideration.
% The main objective of the MIP model is to place a set of cloud VMs among \siteName{s} in a set of subgraphs, such that it can incur minimum VM migrations and power grid usage at runtime caused by the power variability of renewables. 
We now present the VM placement and migration policy of \name{} as the following.
% To identify the optimized solution for VM placement and migration, \name{} makes three decisions: (1) it first decides the suitable subgraph for each VM, (2) then it decides the placement scheme among the \siteName{s} in the subgraph, and (3) finally it makes VM migration decisions to adapt to the power supply changes. 

\begin{table}[t]
    \centering
    \caption{Input constants of the MIP model.}
	\vspace{-1ex}
    \footnotesize{
    \begin{tabularx}{\linewidth}{|c|X|}
        \hline
        Symbol & Interpretation \\
        \hline
        ${\mathbb{M}, \mathbb{N}, \mathbb{K}_n, \mathbb{T}}, t_0$ & A set of $M$ VMs, N subgraphs, $K$ \siteName{s} for subgraph $n$, time interval T, and timestep $t_0$ \\ \hline
        % $Mem_{m}$ & The memory capacity of VM $m$ \\\hline
        $VM\_power_{m}$ & The average power draw of VM $m$ \\\hline
        $Mem_{m}$ & The memory size of VM $m$ \\\hline
        $Lifetime_{m}$ & The predicted lifetime of VM $m$ \\\hline
        $R_{nkt}$ & Renewable power supplied to the $k$th \siteName{s} of subgraph $n$ at time $t$ \\\hline
        $Migr\_Power$ & Power consumption for VM migration per 1GB state \\\hline 
        % $Migr\_out_{m}$ & The extra power needed to migrate out VM $m$ \\\hline
        $Avail\_Target$ & The target availability of VM uptime\\\hline
        % ${\mathbb{M}, \mathbb{N}, \mathbb{K}_n, \mathbb{T}}, t_0$ & A set of M applications, N subgraphs, K \siteName{s} for subgraph $n$, time interval T, and timestep $t_0$ \\ \hline
        % $VM_{m}$ & Number of VMs of application $m$ \\ \hline
        % $Core_{m}$ & Number of cores per VM of application $m$ \\ \hline
        % $Lifetime_{m}$ & Execution time of application $m$ \\ \hline
        % $Supply_{nkt}$ & Power supplied to the $k$th \siteName{s} of subgraph $n$  at time $t$ (in cores) \\ \hline
        % $Migr_{m}$ & Average migration overhead of application $m$ \\ \hline
    \end{tabularx}
    }
    \label{tab:constants}
    \vspace{-3ex}
\end{table}

\noindent \textbf{{VM placement among subgraphs:} }
% As the goal of VM placement is to minimize the impact of power variability and maximize the application performance, we use the average 
% completion time as the main objective in the MIP model (O1 JCT in Equation \ref{eq:subgraph_placement}). 
\name{} relies on heuristic-based approaches for VM placement across subgraphs. This is because the aggregated power supply of each subgraph is relatively stable and hence we empirically find that the heuristic-based approach can well-handle the problem.

\noindent \textbf{{VM placement among \siteName{s} in a subgraph:}}

The main goal of VM placement is to mitigate the impact of power variability on VM interruption with low carbon footprint. Therefore, we define the main objective of the MIP model as minimizing the power grid energy consumption, since it is the main source of operational carbon footprint (O1 in Equation\mbox{~\ref{eq:subgraph_placement}}). We also set a target VM uptime as the lower bound for VM availability (C4). We define the input constants and variables of MIP model in Table~\ref{tab:constants} and~\ref{tab:symbols}, respectively.

%\noindent
%\uline{MIP objective:} The goal of \name{} is to minimize the impact of power variability to applications and maximize their performance. Therefore, we use average application completion time as our main objective (O1 JCT).

\noindent
\uline{MIP input:} 
% %To establish our MIP model, we first need to determine the key input constants (see Table~\mbox{\ref{tab:constants}}). 
% %To achieve the goal of matching application characteristics with the predicted power supply of each subgraph, 
% To map the VMs to the subgraphs with predicted power supply (based on the collected power traces), 
% the MIP model needs to consider three major inputs: (1) application resource requirements, (2) application execution time, 
% and (3) power supply patterns in each subgraph. We quantify the resource requirement for application $m$ using the 
% number of VMs ($VM_m$) required by the application, and the number of cores allocated to each VM ($Core_m$). 
% This is because the resource requirement of an application directly determines the power consumption of \siteName{s}. 
% We can estimate the execution time of application m ($Lifetime_m$) with the historical cloud traces provided by cloud vendors. 
% %which was proven to be practical in the literature~\mbox{\cite{rc, morpheus}}. 
% %We also show that our model 
% %can tolerate mispredictions ($\pm$40\%) of the execution time (\mbox{\S\ref{sec:eval:sensitivity}}). 
% %Finally, 
% We quantify the power supplied to $k$th \siteName{s} in the subgraph $n$ ($Supply_{nkt})$ using the number of 
% CPU cores it can power, based on the power model developed in prior works~\cite{josep:icdcs2014, carbonexplorer:asplos2023}. 
% And the power supply values are predicted one-day ahead using the power production traces. 
The MIP model takes the following input information to help its decision making: 
(1) VM configuration, including its memory size ($Mem_m$) and the number of vCPUs, which can be used to measure its power consumption ($VM\_power_m$);
(2) VM lifetime ($Lifetime_m$); prior work shows that it can be estimated with high accuracy using VM attributes (e.g., VM type, VM size, operating system type) \mbox{\cite{resourcecentral}};
(3) The current power supply of \siteName{s} in each subgraph and the predicted values of future power supply ($R_{nkt}$) (see $\S$\mbox{\ref{sec:predictability}}); 
And (4) the target VM availability ($Avail\_Target$), defined by \mbox{\name} as the average percentage of the VM uptime.

\begin{footnotesize}
\vspace{-1ex}
\begin{align}
\label{eq:subgraph_placement}
\text{O1: NR power} &\quad \text{Minimize} \sum_{n \in \mathbb{N}}\sum_{k \in \mathbb{K}_n}\sum_{t \in \mathbb{T}} NR_{nkt} , \quad \text{\bf s.t.} \\
\text{C1: Power} & \quad \forall n \in \mathbb{N}, t \in \mathbb{T}: \nonumber \\
&\quad \sum_{m \in \mathbb{M}} X_{mnt} \cdot VM\_power_{m} \leq \sum_{k \in \mathbb{K}_n}(NR_{nkt} + R_{nkt}) \nonumber \\
\text{C2: Progress} 
&\quad  V_{mt} = \sum_{n \in \mathbb{N}}\sum_{\tau \le t} (t_0 \cdot X_{mn\tau}) \quad  \forall m \in \mathbb{M}, t \in \mathbb{T} , \quad and \nonumber \\
\text{C3: Completion}  &\quad  V_{mt} \geq Lifetime_{m} \cdot C_{mt}  \quad  \forall m \in \mathbb{M}, t \in \mathbb{T}  , \nonumber \\ 
& \quad  \sum_{t \in \mathbb{T}} C_{mt} = 1, \quad and \nonumber \\
& \quad \sum_{t \in \mathbb{T}} C_{mt} \cdot t = Compl_{m}   \quad \forall m \in \mathbb{M} \nonumber \\ 
\text{C4: Availability}
& \quad Avail_m = \frac{Lifetime_m}{Compl_m}, \quad and \nonumber \\
& \quad \sum_{m \in \mathbb{M}} Avail_m / M \geq Avail\_Target \quad \forall m \in \mathbb{M}  \nonumber \\ \nonumber
\end{align}
\vspace{-6ex}
\end{footnotesize}

% \text{C1: Power} & \quad \forall n \in \mathbb{N}, t \in \mathbb{T}: \nonumber \\
% &\quad \sum_{m \in \mathbb{M}}\sum_{k \in \mathbb{K}_n} (X_{mnkt} \cdot VM\_power_{m} + Migr\_out_m  \cdot \sum_{k_1 \in \mathbb{K}_n} M_{mnk_1k_2t}  + \nonumber \\
% & \quad Migr_m  \cdot \sum_{k_2 \in \mathbb{K}_n} M_{mnk_1k_2t}) \leq \sum_{k \in \mathbb{K}_n}(NR_{nkt} + R_{nkt}) \nonumber \\

\noindent
\uline{MIP output:} 
For VM placement among subgraphs, MIP model denotes placement decisions 
as $X_{mnkt}$ (see Table~\ref{tab:symbols}). It sets $X_{mnkt} = 1$, if application $m$ is assigned to $k$th \siteName{} in subgraph $n$ at time $t$. The second output is denoted as $NR_{nkt}$, which represents the non-renewable power that is supplied to the $k$th \siteName{} in subgraph $n$ at time $t$.

% With the MIP model, \name{} can make optimized placement decisions $X_{mn}$ by aligning the resource requirements $VM_m, Core_m, Lifetime_m$ of the application with the predicted power supplies so as to minimize JCT.

\noindent
\uline{MIP variables and constraints:} We use MIP variables to formulate and track the application states 
(see Table~\mbox{\ref{tab:symbols}}). We list the four major constraints of our MIP model in Equation \ref{eq:subgraph_placement}. 
As the model explores different choices at different timestamps, it has to meet the constraints. 
The first constraint is the power limitation within each subgraph. 
% It indicates that the total number of running cores of all VMs within one subgraph cannot exceed the maximum number of cores allowed by the current power supply $\sum_{k \in \mathbb{K}_n}{NR_{nkt}}$ (C1 Power). 
It indicates that the total power consumption of all VMs cannot exceed the total amount of the power supply from renewable farms and non-renewable power supply from the power grid (C1 Power).
After adding constraint on power limitation, we use two other constraints for defining the VM execution state. 
% By tracking whether an application has sufficient powered VMs for normal execution at each time $t$, 
We keep track of the total uptime of each VM 
$V_{mt}$ (C2 Progress), and when the VM 
uptime $V_{mt}$ reaches its estimated lifetime $Lifetime_m$, 
the model will mark the VM as completed $C_{mt} = 1$ (C3 Completion). To ensure minimized interruption to the VMs, we add one more constraint to the MIP model. The constraint ensures that the average availability (measured by the VM uptime percentage) of all the VMs in~\mbox{\name{}} is higher than the defined target (C4 Availability).

After identifying the suitable subgraph, \name{} further decides where to place the VMs among the \siteName{s} within each subgraph. 
This can be formulated into a similar optimization problem as discussed above. However, we need to additionally consider the power 
variability of each individual \siteName{}, and the potential VM migration overhead (in case the VM has to be migrated, due to the power variability). 
% \hl{
% During the live migration, servers need to allocate additional computing resources to complete the migration, which introduces overhead. The overhead can be categorized into two types~\mbox{~\cite{}}: (1) the higher power usage when VMs migrate into or out of the server, and (2) the performance degradation of VMs. 
% Based on our profiling results (see Figure ~\mbox{~\ref{}}), live migration of a VM can take account $10\%\sim20\%$ extra power. Though live migration will slightly undermine the performance of VMs, it does not significantly impact the overall goal of high availability, so it is disregarded in ~\mbox{\name{}}.
% } 
% Based on our study on the migration overheads of different applications (see $\S$\ref{sec:app-charaterization}),
% we can define the migration sensitivity of cloud applications based on their migration overheads. 
%Based on the different migration overheads observed in different VMs, as shown in Figure~\ref{fig:design:app-characterization} 
%(detailed setup in \S\ref{sec:setup}), we are able to define the migration sensitivity of corresponding VMs. 
Prior work has shown that the VM migration consumes extra power and the power consumption is proportional to the VM memory state transferred through the network~\mbox{\cite{vm_migration_hpdc11}}. We integrate the same power model for VM migration in our MIP model, and we represent the power consumption per 1GB VM state transfer as a constant $Migr\_Power$. In this model, VMs with larger memory states will introduce more migration overhead and are more sensitive to the migration. This can help us align the migration sensitivity of VMs with the power volatility of \siteName{s}.
% For example, the Cofii application has a small migration overhead (which is less sensitive to migrations), 
% while the deep learning (DL) application has a large migration overhead (which is more sensitive to migrations). \zibo{is application profiling needed?}
The MIP model will map migration-sensitive VMs to \siteName{s} having relatively stable energy, and migration-insensitive VMs 
to \siteName{s} that have relatively unstable power sources.  
We now describe how \name{} employs this new insight for the VM placement across \siteName{s} in a subgraph 
by having additional MIP input constants, variables, and constraints.

\begin{table}[t]
    \centering
    \caption{Variables of the MIP model.}
	\vspace{-1ex}
    \footnotesize{
    \begin{tabularx}{\linewidth}{|c|c|X|}
        \hline
        Symbol & Domain & Interpretation \\
        \hline
        $X_{mnt}$ & $\{0, 1\}$ & Whether VM $m$ is powered up in the subgraph $n$ at time $t$ \\\hline
        $Y_{mnkt}$ & $\{0, 1\}$ & Whether VM $m$ is powered up in the $k$th \siteName{} of the subgraph $n$ at time $t$ \\\hline
        $M_{mnk_1k_2t}$ & $\{0, 1\}$ & Whether VM $m$ is migrated from the $k_1$th \siteName{} to the $k_2$th \siteName{} of the subgraph $n$ at time $t$\\\hline
        $NR_{nkt}$ & $\mathbb{R}_{\ge 0}$ & Non-renewable power supplied to the $k$th \siteName{s} of the subgraph at time $t$\\\hline
        $V_{mt}$ & $\mathbb{R}_{\ge 0}$ & The total uptime time of VM $m$ until time $t$\\\hline
        $Compl_{m}$ & $\mathbb{R}_{\ge 0}$ & The actual completion time of application $m$\\ \hline
        % $P_{mt}$ & $\mathbb{R}_{\ge 0}$ & The uptime time of VM $m$ from time $t$ to time $t+1$ \\\hline
        $C_{mt}$ & $\{0, 1\}$ & Whether VM $m$ has completed at time $t$\\ \hline
        $Avail_{m}$ & $[0, 1]$& The percentage of uptime of VM $m$\\\hline
        
        % $V_{mt}$ & $\mathbb{R}_{\ge 0}$ & The valid execution time of application $m$ until time $t$ \\ \hline % check R symbol
        % $S_{mt}$ & $\{0, 1\}$ & Whether application $m$ has sufficient powered VMs running at time $t$ \\ \hline % not aggregated progress
        % $C_{mt}$ & $\{0, 1\}$ & Whether application $m$ has completed at time $t$ \\ \hline
        % $Compl_{m}$ & $\mathbb{R}_{\ge 0}$ & The actual completion time of application $m$\\ \hline
        
        % $X_{mn}$ & $\{0, 1\}$ & Whether application $m$ is assigned to the $n$th subgraph \\ \hline
        % $Y_{mnkt}$ & $\mathbb{N}_{0}$ & The number of VMs of application $m$ placed at the $k$th \siteName{s} of subgraph $n$ at time $t$\\ \hline
        % $M_{mt}$ & $\{0, 1\}$ & Whether application $m$ should migrate at time $t$ \\ \hline
        % $O_{it}$ & $\left[ 0, 1 \right]$ & Overhead of app $i$ at time $t$ \\ \hline
        % $S_{it}$ & $\left[ 0, 1 \right]$ & Migration time of app $i$ at time $t$ \\ \hline % update S with other synbols
        % $R_{it}$ & $\left[ 0, 1 \right]$ & Recomputation overhead of app $i$ at time $t$ \\ \hline
        % $L_{it}$ & $\left[ 0, 1 \right]$ & Latency slowdown of app $i$ at time $t$ \\ \hline
        % $Power_{ijt}$ & $\mathbb{R}_{\ge 0}$ & Power consumed by app $i$ on $j$th site at time $t$ \\ \hline
    \end{tabularx}
	\vspace{-5ex}
    }
    \label{tab:symbols}
\end{table}

% \begin{footnotesize}
% \vspace{-1em}
% \begin{align}
% % \label{eq:subgraph_placement}
% \text{C1': Power} & \quad \forall k \in \mathbb{K}_n, t \in \mathbb{T}: \nonumber \\
% &\quad \sum_{m \in \mathbb{M}} Core_m \cdot VM_m \cdot Y_{mnkt} \cdot S_{mt} \leq Supply_{nkt}  \nonumber \\
% \text{C2': Progress}  &\quad  \sum_{\tau \le t} (S_{m\tau} \cdot t_0 - M_{m\tau} \cdot Migr_m) \leq V_{mt}  \quad  \forall m \in \mathbb{M}, t \in \mathbb{T}  \nonumber \\
% \text{C4: Migration}  &\quad \forall m \in \mathbb{M}, t \in \mathbb{T}: \nonumber \\
% &\quad M_{mt} = \max\{0, \min[1, \max_{k \in \mathbb{K}_n}(Y_{mnkt} - Y_{mnk(t-1)}) ]\}   \nonumber \\ \notag
% \end{align}
% \vspace{-7ex}
% \end{footnotesize}

\begin{footnotesize}
\vspace{-1em}
\begin{align}
% \label{eq:subgraph_placement}
% \text{O1': Nr\_power} &\quad \text{Minimize} \sum_{k \in \mathbb{K}}\sum_{t \in \mathbb{T}} NR_{nkt} \quad \forall n \in \mathbb{N}, \quad \text{\bf s.t.} \\
\text{C1': Power} & \quad \forall n \in \mathbb{N}, \forall k \in \mathbb{K}_n, \forall t \in \mathbb{T}: \nonumber \\
&\quad \sum_{m \in \mathbb{M}} (Y_{mnkt} \cdot VM\_power_{m}) + [\sum_{k_1 \in \mathbb{K}_n} (M_{mnk_1kt} \cdot Mem_m)  + \nonumber \\
& \quad \sum_{k_2 \in \mathbb{K}_n} (M_{mnkk_1t} \cdot Mem_m)] \cdot Migr\_Power \leq NR_{nkt} + R_{nkt} \nonumber \\
\text{C2': Progress}  
% &\quad P_{mt} = t_0 \cdot \sum_{n \in \mathbb{N}}V_{mnt}\quad  \forall m \in \mathbb{M}, t \in \mathbb{T} ,  \nonumber \\
% &\quad  Up_{mt} = \sum_{\tau \le t} P_{m\tau} \quad  \forall m \in \mathbb{M}, t \in \mathbb{T} , \quad and \nonumber \\
&\quad  V_{mt} = \sum_{n \in \mathbb{N}}\sum_{\tau \le t} (t_0 \cdot Y_{mnk\tau}) \quad  \forall m \in \mathbb{M}, \forall k \in \mathbb{K}_n, t \in \mathbb{T} \nonumber \\
\text{C5: Migration} & \quad M_{mnk_1k_2t} \nonumber \\ \nonumber
\end{align}
\vspace{-7ex}
\end{footnotesize}

% \noindent
% \uline{Additional MIP input:} 
% In order to align the VM migration sensitivity to the power variability of \siteName{s}, we introduce the migration overhead $Migr_m$ to the MIP model. 
% \name{} has the migration overheads of cloud applications from cloud vendors (with offline profiling in data centers). 
% To simplify the model execution, we use the average migration overhead of each application as the MIP input.
% \hl{In order to accurately model the impact of the migration, the MIP model takes an additional inputs which represents the additional power consumption needed for VM migration into the server $Migr_m$ and the extra power needed when a VM migrates out of the server $Migr_m$.
% % We use the offline profiled migration overhead (see \mbox{$\S$\ref{sec:app-charaterization}}) as the MIP inputs. 
% These values are compatible compared to the previous studies\mbox{~\cite{}}. 
% }

\noindent
\uline{Additional MIP output:} 
%For application placement across \siteName{s} in a subgraph, 
% The MIP model uses $Y_{mnk(t=0)}$ to 
% denote the application placement decisions across \siteName{s} in a subgraph. $Y_{mnk(t=0)}$ means the number of VMs for application $m$ that will be placed in the $k$th \siteName{} 
% of subgraph $n$ at the time $t=0$ (the point of application deployment).
We add one additional output $M_{mnk_1k_2t}$ to the MIP model, which represent whether a VM $m$ should be migrated from $k_1$th \siteName{} to $k_2$th \siteName{} of subgraph $n$ at time $t$.

\noindent
\uline{Additional MIP variables and constraints:} 
To estimate the total migration overhead of an VM $m$ under power volatility in the MIP model, we will track the events 
when the VMs are migrated. The model will set $M_{mnk_1k_2t} = 1$, if it migrates an VM $m$ at time $t$ (C5 Migration). Once the model detects that an VM needs to be migrated (due to the power changes), 
it will use the variable $M_{mnk_1k_2t}$ and input $Migr\_Power$ to measure its power consumption overhead, 
which affects its total power consumption (C1 Power). 
With these constraints, our MIP model will find an optimized site placement $Y$ for the VMs, with potentially minimal 
migration overheads, which will in turn minimize the total carbon footprint (O1 NR Power).

\noindent \textbf{VM Migration:} \name{} uses the same MIP model as used for VM placement for VM migration, 
since the model has already considered the power variability of sites, VM migration overhead, and VM resource requirements. 
Because VM migration is a dynamic problem, \name{} periodically re-runs the model (once per hour by default) with the new power-supply 
predictions. When \name{} re-runs the MIP model each time, it will set the current timestamp $t$ to be zero. 
We can obtain the VM migration decisions using the difference between the VM placement of the next timestamp 
and the current VM placement $Y_{mnk(t=1)} - Y_{mnk(t=0)}$.

\name{} also periodically re-runs the MIP model to decide how to migrate VMs 
after subgraphs re-identification. The model only considers the \siteName{s} whose corresponding subgraphs have changed. %and the applications whose VMs are located on multiple new subgraphs. 
According to our study, only 30.2\% of the sites change their subgraphs over time, and \name{} re-identifies subgraphs on a weekly basis. 
This will introduce trivial overhead to the overall power consumption.

\noindent\textbf{{Sources of benefits:}}
With the knowledge of VM configuration and the predicted power supply patterns, we expect that MIP model can make optimized decisions by exploiting the following sources of benefits:
(1) VMs that are sensitive to migrations should be placed at \siteName{s} with more stable power supply and insensitive VMs can be placed at less stable \siteName{s}. (2) VMs with longer lifetime should be scheduled to \siteName{s} with longer computation resource availability. (3) We prefer to use non-renewable energy from the power grid for \siteName{s} with unstable renewable power supply or more migration-sensitive VMs. And (4) we prefer to choose migration-insensitive VMs to migrate when possible.

\SetArgSty{textup}
\begin{algorithm}[t]
\footnotesize
\DontPrintSemicolon
\LinesNumbered
 \KwIn{The actual renewable power supply and the VM lifetime\;}
 \KwIn{Power transmission from the grid decided by the MIP model\;}
 \KwResult{}
 Total power supply = Renewable power supply + Transmitted power\;
 \If{Total power supply $\ge$ Power consumption}{
    Misprediction is tolerable;\;
    \KwRet\;
 }
 \uIf{Under-predicted power supply {\normalfont \textbf{or}} over-predicted VM lifetime}{
    \If{\siteName{s} of the same subgraph have remaining energy}{
        Select VMs for migration to other \siteName{s} in descending\;
        order of their average power consumption;\;
    }
    \If{Total power supply < Power consumption}{
        Shutdown VMs to further reduce power consumption\;
        until we reach the target VM uptime;\;
    }
    \If{Total power supply < Power consumption}{
        Transmit more power from the grid to fill the gap;\;
    }
  }
 \Else{
    Misprediction is tolerable;\;
  }
 \caption{Misprediction handling for an \siteName{}.}
 \label{listing:misprediction}
\end{algorithm}
